# Supplementary material for: Risk Assessment Graphs: Utilizing Attack Graphs for Risk Assessment
Source: arXiv:2307.14114 source file (2023-07-26)
Supplement: Supplementary file 1 [file 99_appendix.tex]

% !TEX root = ../AttackGraphBasedRiskAnalysis.tex
% !TEX spellcheck = en_US
% !TEX encoding = UTF-8 Unicode

\section*{Appendix: }\label{appendix}

%\begin{lstlisting}[caption = AND function, numbers = left, breaklines = true, frame = single, firstnumber = 1, language = JavaScript]
\begin{lstlisting}[caption = AND function, breaklines = true, frame = single, firstnumber = 1, language = JavaScript]
function (collection) { 
    var result = {}; 
    collection.childAttributes.forEach(function(child) { 
    for (var attribute in child.attributes) { 
            if (attribute in result) { 
                result[attribute] + = parseInt(child.attributes[attribute]); 
            } else { 
                result[attribute] = parseInt(child.attributes[attribute]); 
            } 
        } 
    }); 
    for (var attribute in result) { 
        if (attribute in collection.globalAttributes) { 
            result[attribute] = Math.min(collection.globalAttributes[attribute].max, result[attribute]); 
        } 
    } 
    return result; 
}
\end{lstlisting}

%\begin{lstlisting}[caption = OR function, numbers = left, breaklines = true, frame = single, language = JavaScript]
\begin{lstlisting}[caption = OR function, breaklines = true, frame = single, language = JavaScript]
function (collection) { 
    var result = null; 
    if (collection.childAttributes.length = = 1) { 
        result = collection.childAttributes[0].attributes; 
    } else { 
        var candidates = []; 
        var worstValue = 0; 
        collection.childAttributes.forEach(function(child) { 
            var value = parseInt(child.computedAttribute); 
            if (value > worstValue) { 
                worstValue = value; 
                candidates = []; 
                candidates.push(child); 
            } else if (value = = worstValue) { 
                candidates.push(child); 
            } 
        }); 
        var tiebreaker = function(candidates, name, max) { 
            var min_value = max; 
            candidates.forEach(function(node) { 
                min_value = Math.min(min_value, node.attributes[name]); 
            }); 
            result = []; 
            candidates.forEach(function(node) { 
                if (node.attributes[name] = = min_value) { 
                    result.push(node); 
                } 
            }); 
            return result; 
        }; 
        if (candidates.length > 1) { 
            candidates = tiebreaker(candidates, "Resources", collection.globalAttributes["Resources"].max); 
            if (candidates.length > 1) { 
                candidates = tiebreaker(candidates, "Knowledge", collection.globalAttributes["Knowledge"].max); 
            } 
        } 
        result = candidates[0].attributes; 
    } 
    return result; 
}
\end{lstlisting}
